# Supplementary material for: VisTW: Benchmarking Vision-Language Models for Traditional Chinese in Taiwan
Source: arXiv:2503.10427 source file (2025-03-15)
Supplement: Supplementary file 1 [file calibration_details.tex]

\section{Calibration}

% [-0.703190647176183, -2.539145833937516, -1.6117171205169678, -1.20832062288082, -1.672244905277005, -3.5341389317943577, 1.4098045357150262, 3.483757951374239, 4.339712022883012, 6.63050528611563, 6.924582905050172]
% 2.999999999999993
