# Supplementary material for: VisTW: Benchmarking Vision-Language Models for Traditional Chinese in Taiwan
Source: arXiv:2503.10427 source file (2025-03-15)
Supplement: Supplementary file 2 [file cover_photo_details.tex]

\section{Traditional Chinese of Figure 1}
\label{app:traditional_chinese_cover}
